# Supplementary material for: Search for the doubly charmed baryon $\it{\Omega}_{cc}^{+}$
Source: arXiv:2105.06841 source file (2021-10-21)
Supplement: Supplementary file 1 [file appendix.tex]

{\noindent\normalfont\bfseries\Large Supplementary materials}
\vspace{0.8em}

\noindent The \Omegacc can decay to \Omegac\pip, where \Omegac decays to \Xicp and \Km. There are few possible \Omegac states, \Omegaca, \Omegacb, \Omegacd, \Omegace and \Omegacf.
To check the contribution from \Omegac\pip, the $m(\Xicp\Km)$ invariant mass distributions after applying Selection A and Selection B 
are shown in Fig.~\ref{fig:XicK_case1} and Fig.~\ref{fig:XicK_case2}.

\begin{figure}[!htp]
  \centering
  \includegraphics[width=0.70\textwidth]{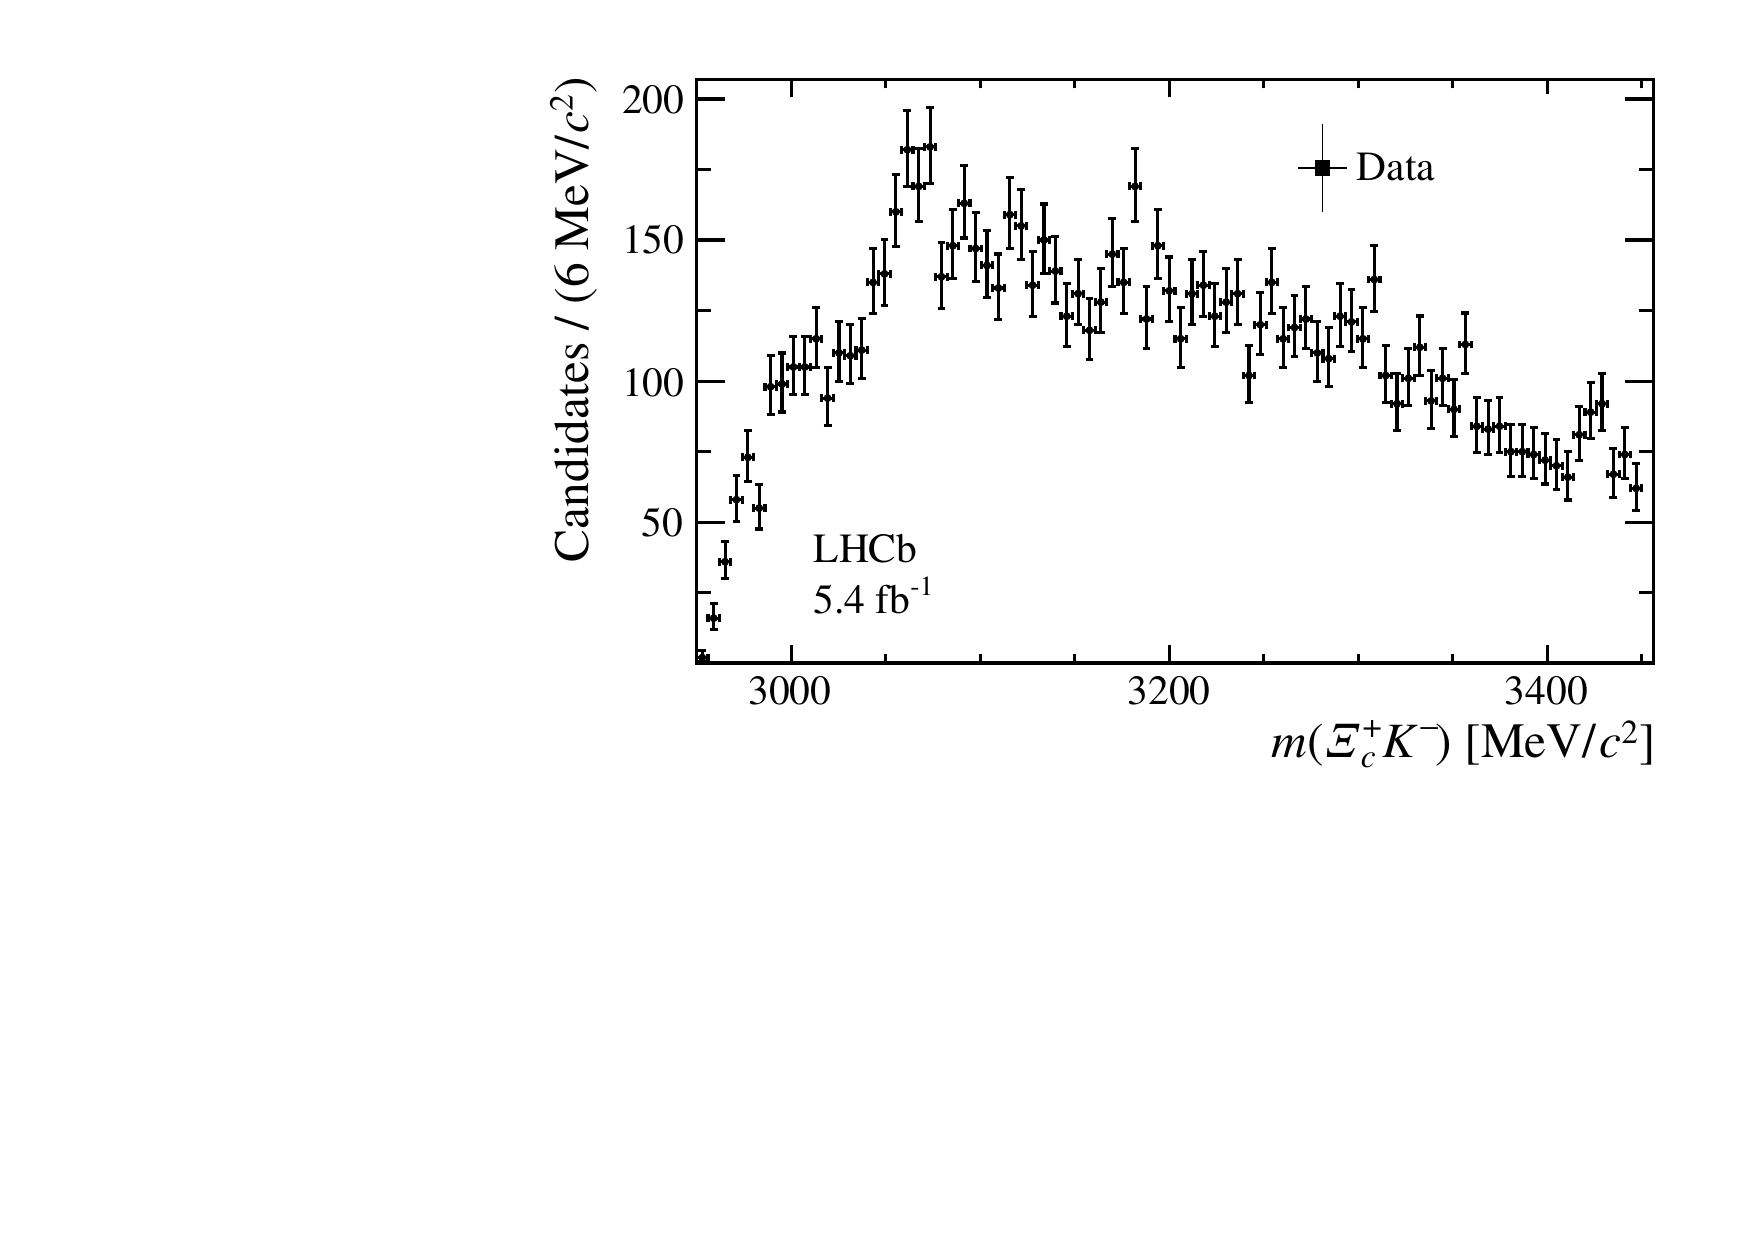}
  \caption{Invariant mass spectrum of \Xicp\Km with selection A.}
  \label{fig:XicK_case1}
\end{figure}

\begin{figure}[!htp]
  \centering
  \includegraphics[width=0.70\textwidth]{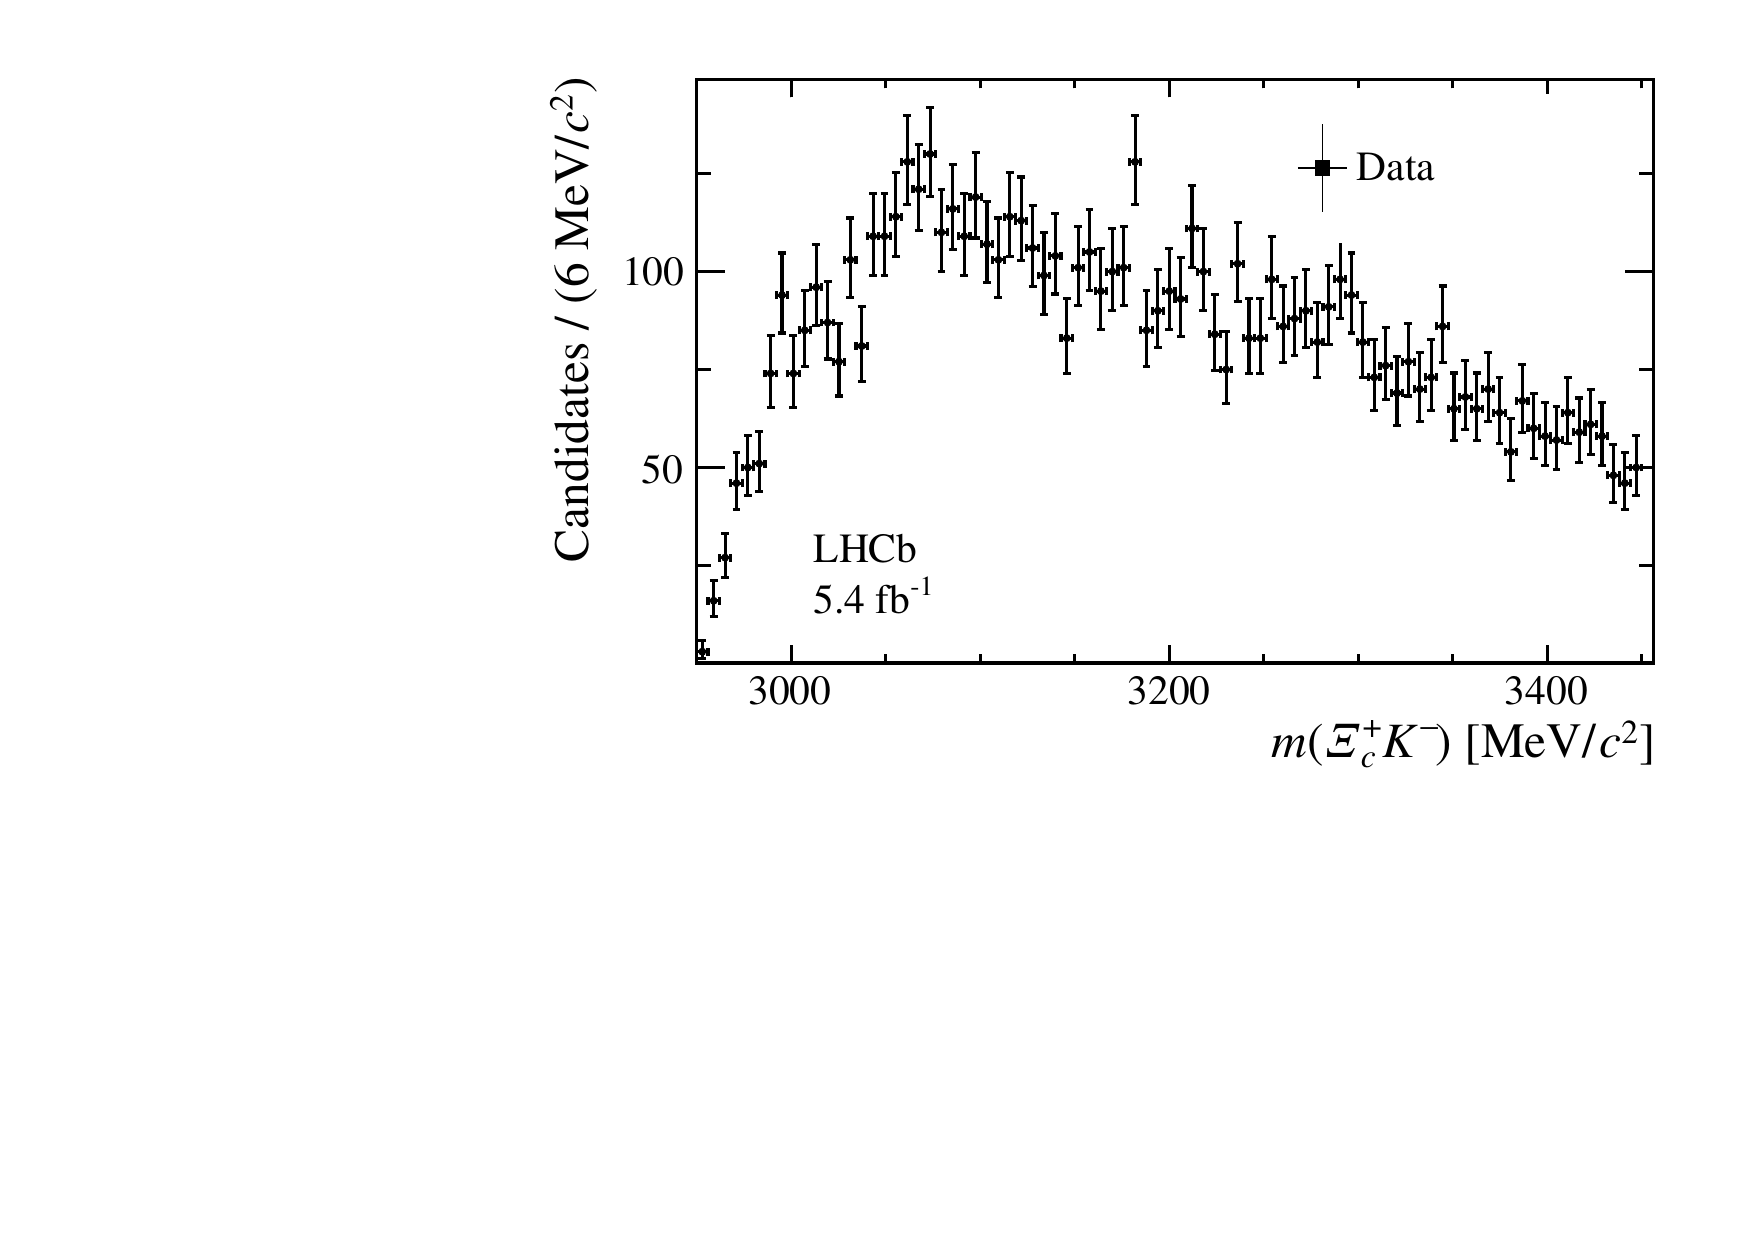}
  \caption{Invariant mass spectrum of \Xicp\Km with selection B.}
  \label{fig:XicK_case2}
\end{figure}

The upper limits on the production ratio $R$ at 90\% credibility level as a function of $m(\Xicp\Km\pip)$ at $\sqrt{s}=13\tev$ is shown in Fig.~\ref{fig:mass_scan_tau_run2_90}.

\begin{figure}[tb]
  \centering
  \includegraphics[width=0.70\linewidth]{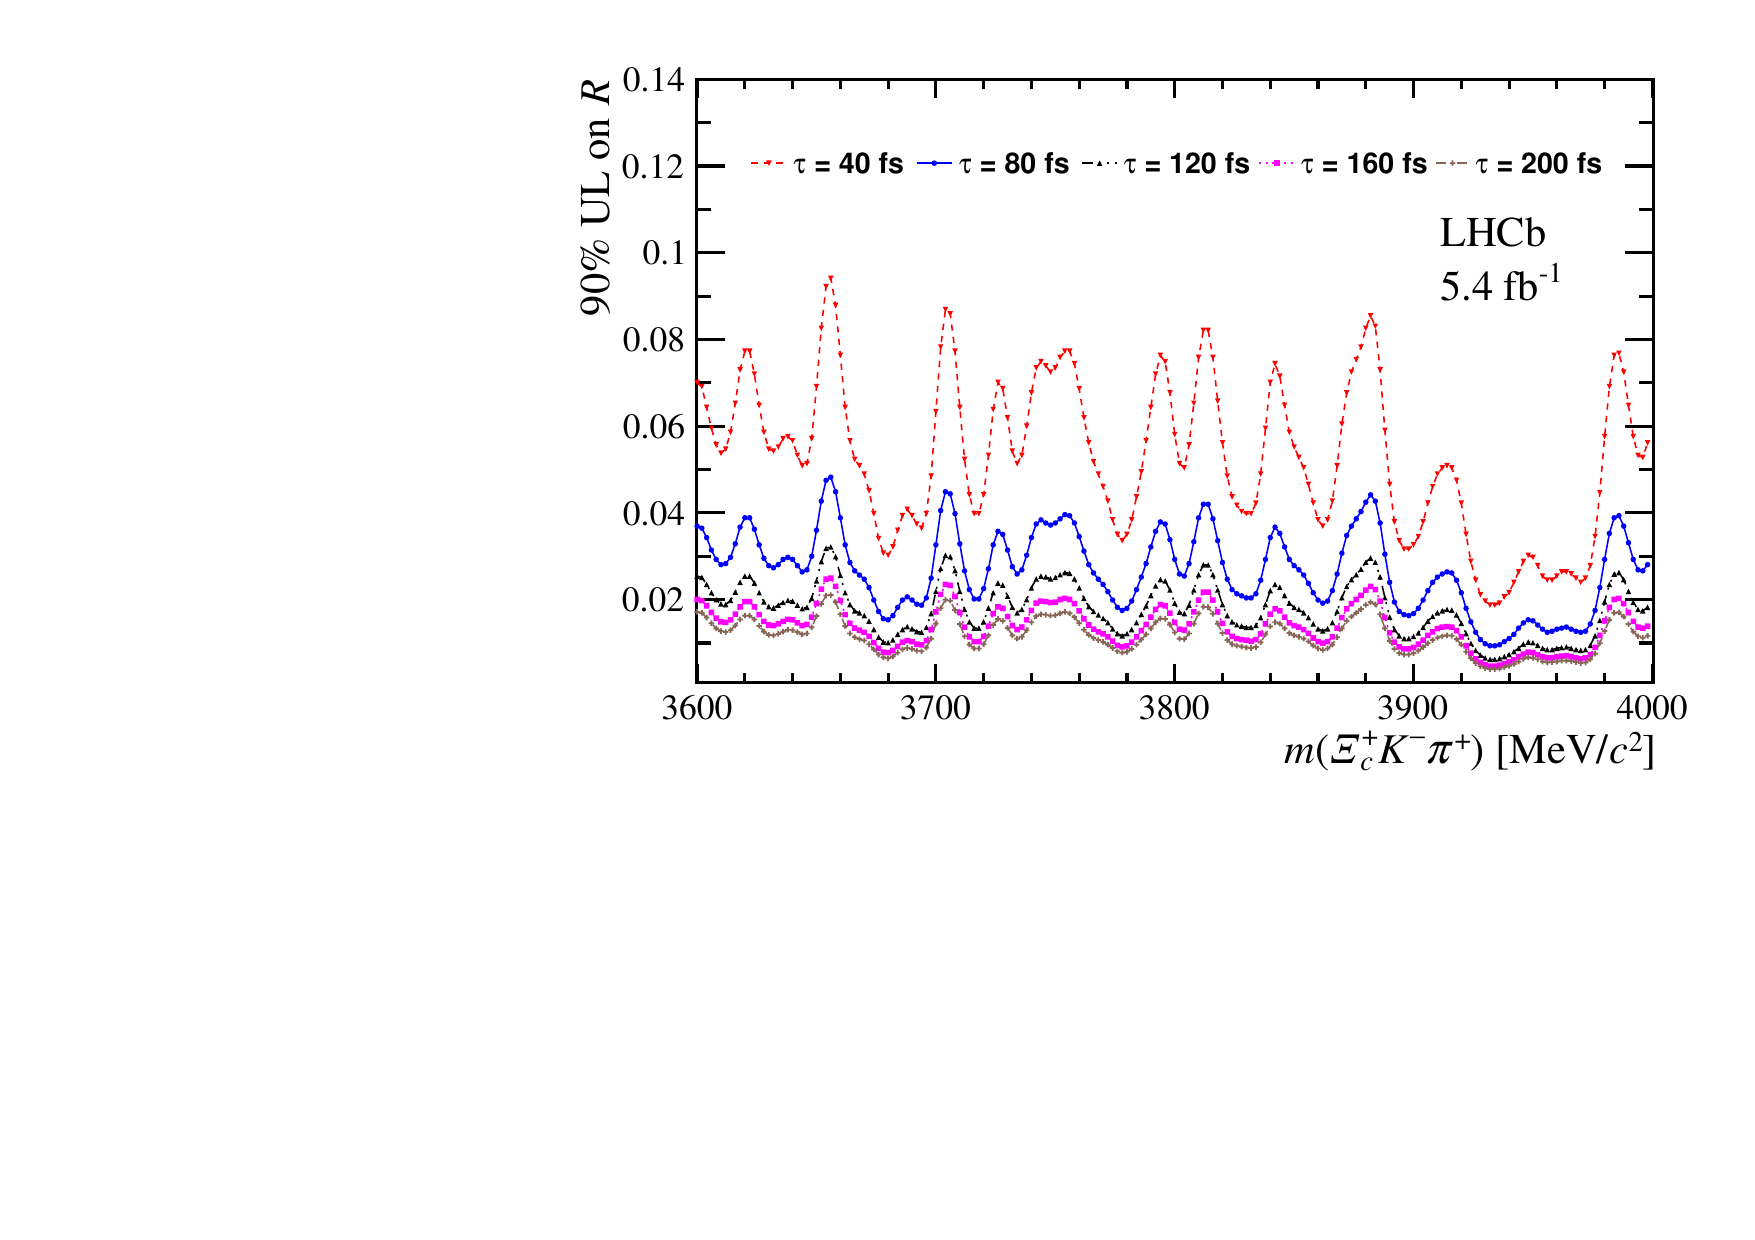}
  \caption{Upper limits on the production ratio $R$
  at 90\% credibility level as a function of $m(\Xicp\Km\pip)$ at
  $\sqrt{s}=13\tev$, 
  for five $\Omegacc$ lifetime hypotheses.}
  \label{fig:mass_scan_tau_run2_90}
\end{figure}
